# Supplementary material for: Fair Exploration via Axiomatic Bargaining
Source: arXiv:2106.02553 source file (2022-07-08)
Supplement: Supplementary file 1 [file app_oam_alg.tex]

%!TEX root=../main_paper.tex

We describe the OAM algorithm from \cite{hao2020adaptive}.

\textbf{Preliminaries: }
Let $G_t = \sum_{s=1}^{t-1} A_s A_s^{\top}$ and let $\htheta_t = G_t^{-1} \sum_{s=1}^{t-1} A_s Y_s$ be the least squares estimate of $\theta$ at time $t$.
Let $\hDelta_t^m(a) = \max_{a' \in \cA(m)} \langle a' - a, \htheta_t \rangle$ be the corresponding estimate of $\Delta^m(a)$.
Let $\hDelta^{\min}_t = \min_{m \in [M]} \min_{a \in \cA(m), \hDelta_t(m, a)>0} \hDelta_t(m, a)$ be the smallest nonzero instantaneous regret.
Let 
\begin{align*}
f_{T, \delta} = 2 \left(1 + \frac{1}{\log T} \right)\log\left(\frac{1}{\delta}\right) + cd \log (d \log T),
\end{align*}
where $c$ is an absolute constant. Let $f_T = f_{T, 1/T}$.

Define the following optimization problem that takes $\tDelta(m, a)$ as input:
\begin{equation}
\begin{aligned} 
\min & \sum_{m \in \cM} \sum_{a \in \cA(m)} Q(m, a) \tDelta(m, a)\\
\text{s.t. } 
\quad
&||a||^2_{H_T^{-1}} \leq \frac{\tDelta(m, a)^2}{f_T} \quad \forall m \in \cM, a \in \cA(m) \\
& Q(m, a) \geq 0  \quad \forall  m \in \cM, a \in \cA,
\end{aligned} 
\tag{$K$} \label{eq:contextual_opt_min_regret_fT}
\end{equation}
where $H_T = \sum_{m \in \cM}\sum_{a \in \cA(m)} Q(m, a) a a^{\top}$ is invertible.
Let $(\hQ_t(m, a))_{m \in \cM, a \in \cA}$ be the solution to \eqref{eq:contextual_opt_min_regret_fT} using $\tDelta = \hDelta_t$.

\textbf{Algorithm: }
We are now ready to state the algorithm.
At each time step $t$, observe context $m_t$ and do the following.
First, check whether
\begin{align} \label{eq:check_constraint_empirical}
||a||^2_{G_t^{-1}} \leq \frac{\hDelta_t(m, a)^2}{f_T} \quad \forall a \in \cA(m_t).
\end{align}
If \eqref{eq:check_constraint_empirical} is satisfied, we exploit; otherwise, we explore.

\noindent \textbf{Exploit: }
Pull the greedy arm: $\argmax_{a \in \cA(m_t)} \langle a, \htheta_t \rangle$.

\noindent \textbf{Explore: }
Let $s(t)$ be the total number of exploration rounds so far.
Solve the empirical optimization problem \eqref{eq:contextual_opt_min_regret_fT} to get solution $\hQ_t(m, a)$.

\begin{enumerate}	
\item Check whether $N_t^{m_t}(a) \geq \min(\hQ_t(m_t, a), f_T / (\hDelta^{\min}_t)^2)$ holds for all available arms $a \in \cA(m_t)$. If so, pull the UCB arm $A_t = \argmax_{a \in \cA(m_t)} \langle a, \htheta_t \rangle + \sqrt{f_{T, 1/s(t)^2}}||a||_{G_t^{-1}}$.
\item Check whether there exists an available arm $a \in \cA(m_t)$ such that $N_t(a) \leq \eps_t s(t)$, where $\eps_t = 1/ \log \log t$.
If there is, then pull $A_t = \argmin_{a \in cA^{m_t}} N_t(a)$.
\item If the above two criteria are not true, then pull $A_t = \argmin_{a \in \cA^{m_t}} \frac{N_t(a)}{\min(\hQ_t(m_t, a), f_T/(\hDelta^{\min}_t)^2)}$.
\end{enumerate}
