# Supplementary material for: Fair Exploration via Axiomatic Bargaining
Source: arXiv:2106.02553 source file (2022-07-08)
Supplement: Supplementary file 2 [file app_warfarin_contextual.tex]

%!TEX root=../neurips_2021.tex

We use a publicly available dataset for warfarin dosing that was collected by the Pharmacogenomics Knowledge Base (PharmGKB \cite{whirl2012pharmacogenomics}), which is under a Creative Commons license\footnote{\url{https://creativecommons.org/licenses/by-sa/4.0/}}.
The dataset contains 5700 patients who were treated with warfarin from 21 research groups over 9 countries. 
Consent for all patients was obtained previously from each center, and no personally identifiable information was used.
The dataset contains the optimal dose of warfarin for each patient, which was found by doctors through trial and error.
It also includes many other covariates for each patient including demographics, clinical features, and genetic information.
% We model this problem as a grouped linear contextual bandit, where we use the race and age of each patient as their group, and other features as their contexts.

\textbf{Groups:}
We group the patients either by race or age.
There were three distinct races in the dataset, which we label as A, B ,and C.
For age, we split the patients into two age groups, where the threshold age was 70.

\textbf{Contexts:}
The OAM and PF-OAM policies assume a finite number of possible feature vectors, and 
the optimization problem \eqref{eq:contextual_opt_min_regret} scales with this number. Therefore, for tractability, we only use five features for the contexts of the patients, where we discretize each feature into two bins.
We use the five features that are most correlated with the optimal warfarin dosage, and we use the empirical median of each feature to discretize them.
The five features that we use are: age, weight, whether the patient was taking another drug (amiodarone), and two binary features capturing whether the patient has a particular genetic variant of genes Cyp2C9 and VKORC1, two genes that are known to affect warfarin dosage \citep{takeuchi2009genome}.
Out of $2^5=32$ different possible feature vectors, there were 21 that were present in the data. 

\textbf{Rewards:}
We bin the optimal dosage levels into three arms as was done in \cite{bastani2020online}: Low (under 3 mg/day), Medium (3-7 mg/day), and High (over 7 mg/day).
To ensure that the model is correctly specified, for each arm, we train a linear regression model using the entire dataset from the five contexts to the binary reward on whether the optimal dosage for that patient belongs in that bin. 
Let $\theta_a \in \bR^6$ be the learned linear regression parameter for each arm ($d=6$ to include the intercept).\footnote{The linear regression step is done solely to remove model misspecification. The purpose of this study is not to show that the linear contextual bandit is a good fit for this dataset --- this was already demonstrated in \cite{bastani2020online}. rather, the purpose is to demonstrate how incorporating fairness changes the outcome from a policy that does not take fairness into account on a bandit instance that approximates a real-world setting.
rather, the purpose is to 
}
To model this as grouped linear contextual bandits as described in \cref{sec:contextual_linear_bandits}, we let $d=18$ and let $\theta = (\theta_{1}, \theta_{2}, \theta_{3}) \in \bR^d$.
When a patient with covariates $X \in \bR^6$ arrives, the actions available are $\{(X, \zerovec, \zerovec), (\zerovec, X, \zerovec), (\zerovec, \zerovec, X)\}$, and their expected reward from arm $a$ is $\langle X, \theta_a \rangle$ for $a \in \{1, 2, 3\}$.

\textbf{Algorithms:}
We assume a patient is drawn i.i.d. from the dataset at each time step, and we compute the asymptotic group regret of the OAM policy (`Regret optimal') and the fair extension (`Fair') as described in \cref{sec:contextual_linear_bandits}:
% \begin{enumerate}[$\circ$]
\begin{itemize}
  \item  \ii{Regret optimal: }
Using the true values $\theta$, we solve \eqref{eq:contextual_opt_min_regret} and obtain solution $(Q(m, a))_{m \in [M], a \in \cA}$.
% The solution gives us $Q(m, a)$ for each context $m$ and arm $a$.
Then, the total (log-scaled) regret incurred by context $m$ is $\sum_{a \in \cA} \Delta(m, a) Q(m, a)$.
Since we assume the group arrivals are i.i.d., for each context, we allocate the regret to groups in proportion to the group's frequency.
That is, for each $m$, let $(w^g(m))_{g \in \cG}$, $\sum_{g \in \cG} w^g(m) = 1$ be the empirical distribution of groups among patients with context $m$.
Then, the total regret assigned to group $g$ is $\sum_{m \in [M]} w^g(m) \sum_{a \in \cA} \Delta(m, a) Q(m, a)$.
\item 
\ii{Fair: }
Using the true values $\Delta$, we solve \eqref{eq:contextual_opt_fair} and obtain solution $(Q^g(m, a))_{g \in \cG, m \in [M], a \in \cA}$.
The total regret assigned to group $g$ is $\sum_{m \in [M]}  \sum_{a \in \cA} \Delta(m, a) Q^g(m, a)$.
% \end{enumerate}
\end{itemize}

All experiments were run on a Macbook Pro with a 2.5 GHz Intel Core i7 processor.
